# Supplementary material for: Taming the time evolution in overdamped systems: shortcuts elaborated from fast-forward and time-reversed protocols
Source: arXiv:2110.03758 ancillary file (2021-10-07)
Supplement: Supplementary file 1 [file SMv3.pdf]

# Supplemental Material for "Taming the time evolution in overdamped systems: shortcuts elaborated from fast-forward and time-reversed protocols"

Carlos A. Plata[1,2], Antonio Prados[2], Emmanuel Trizac[1] and David Guéry-Odelin[3]
[1] *Université Paris-Saclay, CNRS, LPTMS, 91405, Orsay, France*
[2] *Física Teórica, Universidad de Sevilla, Apartado de Correos 1065, E-41080 Sevilla, Spain*
[3] *Laboratoire Collisions, Agrégats, Réactivité, IRSAMC, Université de Toulouse, CNRS, UPS, France*
(Dated: September 1, 2021)

We present in Section I different simple prescriptions that provide admissible protocols. Nevertheless, all of them are limited either by the specificity of the particular case or by impossibility of writing the protocol in closed-form. This underscores the interest of the different route worked out in the main text: generic and explicit. We then address in Section II the continuity of the driving potential at the final time of the steering, a key feature for the success of the welding idea. In section III, we address the important question of the protocol cost, and discuss optimal features. The relationship between the intensity of the required driving and the velocity of the process, given by the finite duration of the protocol, is analyzed. We also study the consequences on the protocol speed of a maximal possible force (in absolute value), a situation met in experiments. Section IV is devoted to two analytically solvable problems and to the optimal connection between Gaussian states, while the spectral results needed are presented in section V. The resulting expansions may be truncated, which leads to some error, analyzed in section VI. Generalizations to higher dimensions are finally discussed in section VII.

## I. TOWARDS EXPLICIT PROTOCOLS: PARTICULAR EXAMPLES, INTERPOLATION PRESCRIPTION, AND SHAPE-PRESERVING DYNAMICS

Equation (2) in the main text gives the force required for driving the system through a prescribed and arbitrary time evolution $\rho(x,t)$. In our work, we have chosen this prescription to be the time-manipulated version of a reference process. However, numerous prescriptions are possible. Herein, we provide three different choices. Namely, we present (i) some particular examples motivated by the few explicit protocols already present in the literature, (ii) an interpolation prescription, and (iii) a shape preserving dynamics. The first one reproduces and partially generalizes some specific protocols, the second one provides a solution—which is not expressible in closed form in general—for arbitrary connections, whereas the last one makes it possible to write simple solutions for shape-preserving connections.

For the sake of a neater presentation, we rewrite Eq. (2) of the main text in terms of the cumulative distribution function

$$R(x,t) = \int_{x_b}^{x} dx' \rho(x,t), \tag{S1}$$

instead of the probability distribution $\rho(x,t)$. Therefore, in this section, we will use

$$\partial_x U(x,t) = -\beta^{-1}\partial_x \ln\left[\partial_x R(x,t)\right] + \gamma \frac{\partial_t R(x,t)}{\partial_x R(x,t)}. \tag{S2}$$

As a consequence, any admissible derivable cumulative distribution function $R(x,t)$ provides us with a driving force in closed form that makes the desired connection.

All explicit protocols obtained hitherto in the literature, which are just a few [1–4], can be derived either by substituting a simple prescription for $R(x,t)$ in Eq. (S2) or by using directly the property of shape-preserving processes derived below.

### A. Particular protocols

We start by introducing two specific examples discussed in Refs [3, 4]. Both of them are finite time processes, $t \in [0, t_\mathrm{f}]$, described in a finite space, $x \in [0, L]$ which end up at the homogeneous distribution $\rho_\mathrm{f}(x) = 1/L$ featuring an optimal mean work, defined in the framework of stochastic thermodynamics, along the process—see also Sec. III. Here, we consider dimensionless variables, $t_\mathrm{f} = 1$ and $L = 1$, for consistency with the results in Refs. [3, 4]. Zhang explicitly obtained the optimal connection—in the sense of minimizing the irreversible work—between two different initial distributions, namely

$$\rho_\mathrm{i}^{(I)}(x) = \frac{1}{\sqrt{4x}} \qquad \text{and} \qquad \rho_\mathrm{i}^{(II)}(x) = 2x, \tag{S3}$$

and the final homogeneous distribution $\rho_{\rm f}(x) = 1$. The solutions for the respective optimal connections are

$$\rho^{(I)}(x,t) = \frac{1}{\sqrt{t^2 + 4(1-t)x}} \qquad \text{and} \qquad \rho_{\rm i}^{(II)}(x,t) = \frac{1}{t} + \frac{t-1}{t\sqrt{(1-t)^2 + 4tx}}, \tag{S4}$$

which can be enforced by the driving potential obtained from our reverse-engineering procedure.

In the following, we work out a generalization of the process labelled by (I) where optimality is not compelled, allowing more flexibility. In particular, we propose the prescription

$$\rho(x,t) = \mathcal{N}(t)[\xi(t)^2 + 4(1-\xi(t))x]^{\alpha} \tag{S5}$$

for the density, where $\xi(t)$ is an increasing function fulfilling $\xi(0) = 0$, $\xi(1) = 1$, $\alpha > -1$ is a real parameter, and the factor

$$\mathcal{N}(t) = \frac{4(1+\alpha)[1-\xi(t)]}{\{\xi(t)^2 + 4[1-\xi(t)]\}^{1+\alpha} - \xi(t)^{2(1+\alpha)}} \tag{S6}$$

ensures the normalization of the density. This provides a broader class of connections to the homogeneous distribution, than that subsumed in Eq. (S4). Note that for $\alpha = -1/2$ and $\xi(t) = t$, we recover the optimal process of [4]. In the following section we present an alternative to this pathway, introducing a linear interpolation between the initial and target states. The cumulative distribution function corresponding to the prescription given in Eq. (S5) can be explicitly obtained,

$$R(x,t) = \mathcal{N}(t)\frac{\{\xi(t)^2 + 4[1-\xi(t)]x\}^{1+\alpha} - \xi(t)^{2(1+\alpha)}}{4(1+\alpha)[1-\xi(t)]}. \tag{S7}$$

Therefore, by substituting Eq. (S7) into Eq. (S2) we get

$$\partial_x U(x,t) = -\beta^{-1}\alpha\frac{4[1-\xi(t)]}{\xi(t)^2 + 4[1-\xi(t)]x} + \frac{\gamma\dot{\xi}(t)}{4(1+\alpha)[1-\xi(t)]^2} \tag{S8}$$

$$\times\left\{2(1+\alpha)\xi(t) - 4\alpha[1-\xi(t)]x - (1+2\alpha)\xi(t)^2 - \xi(t)^{1+2\alpha}\frac{1 + (1+2\alpha)[1-\xi(t)]}{\{\xi(t)^2 + 4[1-\xi(t)]x\}^{\alpha}}\right\}, \tag{S9}$$

and the driving potential is

$$U(x,t) = -\beta^{-1}\alpha\ln\left\{\xi(t)^2 + 4[1-\xi(t)]x\right\} + \frac{\gamma\dot{\xi}(t)}{16(1-\alpha^2)[1-\xi(t)]^3} \tag{S10}$$

$$\times\left[4(1-\alpha)[1-\xi(t)]x\left\{2(1+\alpha)\xi(t) - 2\alpha[1-\xi(t)]x - (1+2\alpha)\xi(t)^2\right\} - \xi(t)^{1+2\alpha}\frac{1+(1+2\alpha)[1-\xi(t)]}{\{\xi(t)^2 + 4[1-\xi(t)]x\}^{\alpha-1}}\right], \tag{S11}$$

defined up to an additive arbitrary function of time. This procedure gives neither a very illuminating nor a simple protocol. In the next section, we use an interpolation approach to give a general recipe to connect distributions explicitly, provided that the distribution have a closed-form cumulative distribution functions. Specifically, we employ our result to connect states which are proportional to an arbitrary power of $x$.

### B. Interpolation prescription

We discuss here a different approach, which has been used in the context of fast driving of quantum systems [5]. It consists of a linear interpolation between the initial and final states, $\rho_{\rm i}(x)$ and $\rho_{\rm f}(x)$, in the form

$$\rho(x,t) = s(t)\rho_{\rm i}(x) + [1-s(t)]\rho_{\rm f}(x), \tag{S12}$$

where $s(t)$ is a function that varies from $s(0) = 1$ to $s(t_{\rm f}) = 0$ in the time interval $[0, t_{\rm f}]$. Interpolation at the level of probability density functions entails the same relation in its cumulative distribution functions

$$R(x,t) = s(t)R_{\rm i}(x) + [1-s(t)]R_{\rm f}(x), \tag{S13}$$

with $R_{\rm i}(x)$ and $R_{\rm f}(x)$ standing for the initial and final cumulative distribution functions, respectively. Substituting Eq. (S13) into Eq. (S2), we get

$$\partial_x U(x,t) = -\beta^{-1}\partial_x \ln\left[\partial_x R(x,t)\right] + \gamma\dot{s}(t)\frac{R_{\rm i}(x)-R_{\rm f}(x)}{\partial_x R(x,t)}. \tag{S14}$$

The departure of the potential to be applied from its quasistatic form is then quantified by the last term on the rhs of Eq. (S14). If we want to start from equilibrium with $U(x,0)=U_i(x)$ and arrive at equilibrium with $U(x,t_{\rm f})=U_{\rm f}(x)$, we may need a time discontinuous potential. More specifically, if $\dot{s}\neq 0$, we have $U(x,0^+)\neq U_i(x)$ and $U(x,t_{\rm f}^-)\neq U_{\rm f}(x)$ at both the initial and final times.

The practical usefulness of such a procedure to obtain a driving force in closed-form depends on the existence of analytical expressions for the cumulative distribution functions. In other words, it depends on the existence of analytical expressions for the primitives of $\rho_{\rm i}(x)$ and $\rho_{\rm f}(x)$. Otherwise, this method does not lead to explicit results for connecting the initial and final states, at variance with the welding method in the main text (exemplified therein with the example of the connection between $x^4$ and $x^6$ potentials).

Let us illustrate the interpolation approach for the connection between the initial and final distributions

$$\rho_{\rm i}(x) = \frac{1+\alpha_{\rm i}}{L^{1+\alpha_{\rm i}}}x^{\alpha_{\rm i}} \qquad \text{and} \qquad \rho_{\rm f}(x) = \frac{1+\alpha_{\rm f}}{L^{1+\alpha_{\rm f}}}x^{\alpha_{\rm f}}, \tag{S15}$$

for $x\in[0,L]$. The cumulative distribution functions are simple to compute:

$$R_{\rm i}(x) = \left(\frac{x}{L}\right)^{1+\alpha_{\rm i}} \qquad \text{and} \qquad R_{\rm f}(x) = \left(\frac{x}{L}\right)^{1+\alpha_{\rm f}}, \tag{S16}$$

which allows us to obtain the required driving force as

$$\partial_x U(x,t) = -\beta^{-1}\partial_x \ln\left\{s(t)\frac{1+\alpha_{\rm i}}{L^{1+\alpha_{\rm i}}}x^{\alpha_{\rm i}} + [1-s(t)]\frac{1+\alpha_{\rm f}}{L^{1+\alpha_{\rm f}}}x^{\alpha_{\rm f}}\right\} + \gamma\dot{s}(t)\frac{\left(\frac{x}{L}\right)^{1+\alpha_{\rm i}} - \left(\frac{x}{L}\right)^{1+\alpha_{\rm f}}}{s(t)\frac{1+\alpha_{\rm i}}{L^{1+\alpha_{\rm i}}}x^{\alpha_{\rm i}} + [1-s(t)]\frac{1+\alpha_{\rm f}}{L^{1+\alpha_{\rm f}}}x^{\alpha_{\rm f}}}. \tag{S17}$$

The above approach provides an alternative to the connection between the initial and final states derived in the previous section.

### C. Shape-preserving dynamics and their simple driving potential

Let us assume a shape-preserving dynamics, that is,

$$\rho(x,t) = \frac{\exp\left[-\beta U_{\rm i}\left(\frac{x-\mu(t)}{\sigma(t)}\right)\right]}{\sigma(t)Z_{\rm i}}, \tag{S18}$$

with $\mu(t)$ and $\sigma(t)$ being continuous real functions such that $\mu(0)=0$ and $\sigma(0)=1$, and $Z_{\rm i}=\int_{\mathcal{D}} dx\, e^{-\beta U_{\rm i}(x)}$ the partition function guaranteeing the correct normalization of the distribution. Such a situation is restrictive, in the sense that it connects distributions of the same family, but also general, in the sense that the shape of the potential $U_i(x)$ is completely arbitrary. In particular, the final potential must fulfill

$$U_{\rm f}(x) = U_{\rm i}\left(\frac{x-\mu(t_{\rm f})}{\sigma(t_{\rm f})}\right). \tag{S19}$$

We can obtain the driving needed to produce this shape preservation by introducing Eq. (S18) into Eq. (S2),

$$\partial_x U(x,t) = \partial_x U_{\rm i}\left(\frac{x-\mu(t)}{\sigma(t)}\right) - \gamma\frac{\dot{\mu}(t)\sigma(t)+[x-\mu(t)]\dot{\sigma}(t)}{\sigma(t)}, \tag{S20}$$

which derives from the potential

$$U(x,t) = U_{\rm i}\left(\frac{x-\mu(t)}{\sigma(t)}\right) - \gamma\frac{2\dot{\mu}(t)\sigma(t)[x-\mu(t)]+[x-\mu(t)]^2\dot{\sigma}(t)}{2\sigma(t)}. \tag{S21}$$

For obtaining the driving, we have made use of the following: (i) the location of the boundary at infinity, since strictly shape-preserving dynamics entails that the domain is the whole real line and, consequently, (ii) the cumulative distribution function of the shape-preserving dynamics fulfilling $R(x,t) = R_{\mathrm{i}}\left(\frac{x-\mu(t)}{\sigma(t)}\right)$, where $R_{\mathrm{i}}(x)$ is the cumulative distribution function at the initial time.

Equation (S21) implies that the potential required to drive a system featuring shape preservation involves two contributions. One of them is the shape-bearing potential itself while the other is a harmonic potential with stiffness and center determined by certain combinations of the shift and scaling functions $\mu(t)$ and $\sigma(t)$. Remarkably, the property of shape preservation makes it possible to always write an explicit solution for the potential, even for densities $\rho(x,t)$ for which the corresponding cumulative distribution functions $R(x,t)$ do not have an analytical expression. If one is exclusively interested in smooth protocols, vanishing $\dot{\mu}(t)$ and $\dot{\sigma}(t)$ at both the initial and final times should be considered.

## II. (DIS)CONTINUITY AT FINAL TIME DEPENDING ON $\Lambda(t)$

In Eq. (11) of the main text, we have obtained that, when considering the acceleration of infinite-time processes, i.e., $\lim_{t\to t_{\mathrm{f}}}\Lambda(t) = +\infty$, the behavior $\partial_x \Delta U(x,t)$ is dominated by $\frac{de^{-\lambda_1\Lambda(t)}}{dt}$, with $\lambda_1$ the smallest eigenvalue that characterizes the relaxation process. Can the resulting behavior when $t\to t_{\mathrm{f}}^-$ be singular? To identify the critical case that separates 0 from $-\infty$ for the (negative) derivative in question, we introduce a constant $C<0$ such that

$$\frac{de^{-\lambda_1\Lambda_c(t)}}{dt} \sim C, \quad t\to t_{\mathrm{f}}^-. \tag{S22}$$

Integrating between $t$ and $t_{\mathrm{f}}$, this implies

$$e^{-\lambda_1\Lambda_c(t)} \sim -C(t_{\mathrm{f}}-t). \tag{S23}$$

Therefore,

$$-\lambda_1\Lambda_c(t) \sim \ln(-C) + \ln(t_{\mathrm{f}}-t) \tag{S24}$$

or

$$\Lambda_c(t) \sim -\frac{\ln(t_{\mathrm{f}}-t)}{\lambda_1}, \quad t\to t_{\mathrm{f}}^-. \tag{S25}$$

In this "critical" case, the force displays a finite jump at $t_{\mathrm{f}}$.

On the one hand, if $\Lambda(t)$ diverges at $t_{\mathrm{f}}^-$ faster than $\Lambda_c(t)$, we have that the exponential goes to zero faster than in the critical case and therefore $\Delta U\to 0$, which is the "regular" case considered in the main text. For instance, the family of algebraic power laws given in Eq. (6) belongs in this category. On the other hand, if $\Lambda(t)$ diverges at $t_{\mathrm{f}}^-$ slower than $\Lambda_c(t)$, we have that the exponential goes to zero slower than in the critical case and therefore $\Delta U\to\infty$ (the "singular" case). Very slowly diverging $\Lambda$-functions, such as $\sqrt{-\ln(t_{\mathrm{f}}-t)}$ or $\ln[-\ln(t_{\mathrm{f}}-t)]$, belong in here. The rationale behind this discrimination (fast/slow divergence) is that for slowly diverging $\Lambda(t)$, large values of $\Lambda$ are met only for $t$ very close to $t_{\mathrm{f}}$. This means that a significant fraction of the evolution needs to be performed in a too narrow time window in the vicinity of $t_{\mathrm{f}}$, which requires strong (and actually divergent) forces. With a more quickly divergent $\Lambda(t)$, the time window in question is extended, with a concomitant decrease of the required forces.

We note that the conclusions reached in this derivation for forward processes at the final time can be directly translated to time-reversed processes at the initial time. As stated in the main text, Eq. (5) guarantees the continuity of the force field at the initial (final) time when $\dot{\Lambda}$ vanishes thereat in forward (backward) processes.

## III. FASTER PROTOCOLS ENTAIL HIGHER COST. OPTIMAL CONNECTIONS

### A. Maximum exerted force

From Eq. (5) of the main text, we can derive the asymptotic behavior of the driving for either very slow or fast connections. In the limit where $t_{\mathrm{f}}\to\infty$, we have that $\dot{\Lambda}(t)\to 0$ and

$$\partial_x U(x,t) \sim -\beta^{-1}\partial_x \ln\rho_{\mathrm{r}}(x,\Lambda(t)). \tag{S26}$$

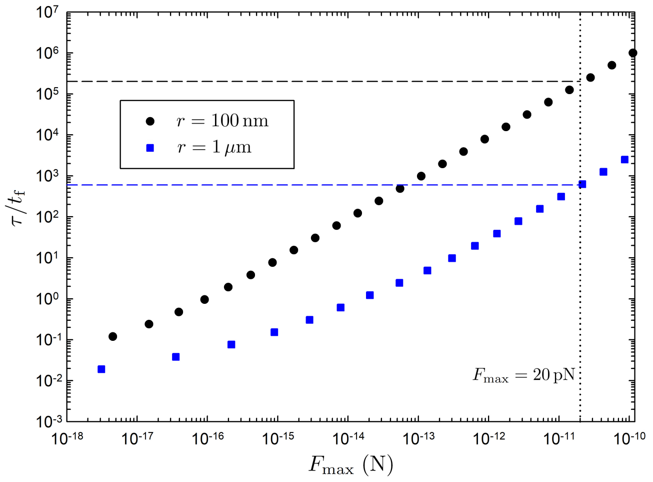


FIG. S1. Acceleration factor in the fast-forward procedure as a function of the maximum force exerted. The protocol is that presented in Fig. 2, and two colloidal sizes have been considered. The factor of acceleration obtained when the maximum force is 20 pN (vertical dotted line) is highlighted by a horizontal dashed line. The dependence is linear with slope 1 in log-log scale for short time (large forces) showing that the maximum force scales as $t_{\mathrm{f}}^{-1}$, as theoretically predicted.

For such a slow connection, the evolution sweeps equilibrium states driven by the unperturbed "quasistatic" potential $-\beta^{-1}\partial_x \ln \rho_{\mathrm{r}}(x, \Lambda(t))$. For fast connections, i.e., in the limit $t_{\mathrm{f}} \to 0$, the driving force becomes

$$\partial_x U(x,t) \sim \dot{\Lambda}(t)\partial_x[U_{\mathrm{r}}(x) + \beta^{-1}\ln \rho_{\mathrm{r}}(x, \Lambda(t))]. \tag{S27}$$

The driving is proportional to the difference between the reference potential and the "quasistatic" potential with factor of proportionality $\dot{\Lambda}(t)$. Furthermore, our choice for $\Lambda(t) = \tau f(t/t_{\mathrm{f}}) = g(t/t_{\mathrm{f}})$ makes it particularly simple to study the dependence on $t_{\mathrm{f}}$, since $\dot{\Lambda}(t) = t_{\mathrm{f}}^{-1} g'(t/t_{\mathrm{f}})$. Henceforth, we obtain that shorter $t_{\mathrm{f}}$ lead, in absolute value, to higher forces scaling as $t_{\mathrm{f}}^{-1}$ as $t_{\mathrm{f}} \to 0$.

If experimental conditions are limited to forces below a certain maximum, Eq. (5) of the main text constrains the minimum time for feasible connections. Here, we analyze the effect of such a constraint in the sedimentation example illustrated in Fig. 2. We have plotted in Fig. S1, the acceleration factor $\tau/t_{\mathrm{f}}$, with $\tau = \lambda_1^{-1}$ being the characteristic relaxation time of the reference process, as a function of $F_{\max}$, the maximum force required during the fast-forward protocol. We assume that these particles, spheres of radius $r$, have mass density comparable to that of water ($10^3\,\mathrm{kg/m^3}$), and are confined in a cell of width $L = 4r$, in the direction aligned with the gravitational field. The colloidal particles feel (i) the constant gravitational force that produces an acceleration of $9.8\mathrm{m/s^2}$ plus (ii) the optical force $-\partial_x U$ we can manipulate in order to implement the fast-forward protocol. Considering typical room temperature $T = 300\,\mathrm{K}$, we obtain the two set of values shown in Fig. S1 for particles of radius $r = 100\,\mathrm{nm}$ and $r = 1\,\mu\mathrm{m}$, which are typical sizes for colloidal particles. Assuming $F_{\max} = 20\,\mathrm{pN}$, typical value when using optical traps [6], we obtain that the minimum connection time reachable are $\tau/t_{\mathrm{f}} \simeq 2 \times 10^5$ and $\tau/t_{\mathrm{f}} \simeq 6 \times 10^2$. Both imply a significant acceleration with respect to the free relaxation.

The above values for the minimum time $t_{\mathrm{f}}$ are conditioned to a given choice for the time manipulation function $\Lambda(t)$ or, equivalently, for $g(t/t_{\mathrm{f}})$. One may look for smarter protocols, that would minimize the maximum force required, for a given $t_{\mathrm{f}}$. This raises the generic question of optimal properties, addressed in the next section with a different aim. We shall discuss there the conditions under which the fast-forward protocol minimizes the work dissipated during the process.

### B. Minimum dissipated work

Herein, we minimize the cost of the fast-forward protocol, as measured by the average work carried out during the transformation: for a given reference potential $U_r$, we seek the optimal function $\Lambda(t)$. Thus, the sequence of states in between the initial and final states is prescribed, given by the reference dynamics, while the "speed" at which such sequences are visited is not constrained, and ruled by $\Lambda(t)$. As a consequence, the present optimization problem does not coincide in general with the "full optimum", where arbitrary states can be visited at intermediate times.

To put is short, one optimizes over eligible functions $\Lambda(t)$ for finding the optimal fast-forward protocol, while the full optimum requires also optimization with respect to $U_{\rm r}$. It is understood here that the initial and final states are prescribed/given.

The average work is

$$W=\int_0^{t_{\rm f}} dt\,\langle\partial_t U(x,t)\rangle=\int_0^{t_{\rm f}} dt\int_{\mathcal{D}} dx\,\partial_t U(x,t)\rho(x,t), \tag{S28}$$

which can be split into two contributions,

$$W=\Delta F+W^{\rm (irr)},\quad \Delta F=-\beta^{-1}\ln\frac{\int dx e^{-\beta U_{\rm f}(x)}}{\int dx\, e^{-\beta U_{\rm i}(x)}},\quad W^{\rm (irr)}=\gamma\int_0^{t_{\rm f}} dt\int_{\mathcal{D}} dx v^2(x,t)\rho(x,t). \tag{S29}$$

Here, $\Delta F$ stands for the free energy change and $W^{\rm (irr)}\geq 0$ is the irreversible (or excess) work. The former depends solely on the initial and final states, whereas the latter is a functional of the whole protocol through the velocity field $v(x,t)\equiv-\gamma^{-1}\left[\partial_x U(x,t)+\beta^{-1}\partial_x\ln\rho(x,t)\right]$.

In the main text, we have expressed the potential required for performing a fast-forward transformation in terms of the velocity field of the reference process. For our present purposes, writing the relation between the velocity fields in the fast-forward protocol and the reference process is more useful. By using the definition of the velocity field and Eq. (5), we get

$$v(x,t)=\dot\Lambda(t)v_{\rm r}(x,\Lambda(t)). \tag{S30}$$

Taking into account that the time contraction/dilation function is a function of $s=t/t_{\rm f}$, $\Lambda(t)=g(t/t_{\rm f})$, we can write

$$W^{\rm (irr)}=\frac{1}{t_{\rm f}}\int_0^1 ds\, g'(s)^2\underbrace{\gamma\int_{\mathcal{D}} dx\, v_{\rm r}^2(x,g(s))\rho_{\rm r}(x,g(s))}_{\mathcal{P}_{\rm r}^{\rm (irr)}(g(s))}. \tag{S31}$$

The underbraced quantity is the production rate of the irreversible work in the reference process, i.e., the irreversible power [7]. The irreversible work scales as $1/t_{\rm f}$: shorter connections go with enhanced irreversible work.

Let us consider a fixed connection time $t_{\rm f}$ and ask ourselves what is the fast-forward protocol, as determined by $g(s)$, that minimizes the irreversible work. This is a well-posed minimization problem: although the irreversible power for the reference process $\mathcal{P}_{\rm r}^{\rm (irr)}$ may be cumbersome, it is a known function. Writing down the Euler-Lagrange equation associated to the functional under scrutiny, we get the differential equation that determines the optimal choice for $g(s)$,

$$2g''(s)\mathcal{P}_{\rm r}^{\rm (irr)}(g(s))+\mathcal{P}_{\rm r}^{\rm (irr)\prime}(g(s))g'(s)^2=0, \tag{S32}$$

which has to be supplemented with proper boundary conditions. Specifically, our fast-forward of an infinite reference relaxation process imposes $g(0)=0$ and $\lim_{s\to 1} g(s)=\infty$. Note that Eq. (S32) can be analytically integrated once, obtaining the first integral

$$g'(s)^2\,\mathcal{P}_{\rm r}^{\rm (irr)}(g(s))=C>0 \tag{S33}$$

where $C$ is a constant. This first integral of motion is a remarkable property: it indicates that the rate at which the dissipated work increases is constant over the optimal fast-forward protocol. Inserting Eq. (S33) into (S31), one gets

$$W^{\rm (irr)}=\frac{1}{t_{\rm f}}C \implies C=t_{\rm f}W^{\rm (irr)}=t_{\rm f}^2\mathcal{P}^{\rm (irr)}. \tag{S34}$$

Interestingly, it has been shown that the dissipated power is also constant for the "full" optimization problem, i.e., when a completely arbitrary connection between the initial and final states is considered [3, 8–10].

The solution to (S32) provides us with the optimal fast-forward connection. The function $\mathcal{P}_{\rm r}^{\rm (irr)}$ depends on the reference process considered, i.e., on $U_{\rm r}$; so does the optimal fast-forward protocol. As emphasized above, since we are carrying out the optimization over a certain, limited, family of shortcuts—those of fast-forward type, we cannot guarantee that our optimal fast-forward connection coincides with the full optimal one—i.e., considering all the possible processes. Nevertheless, in Section IV C, we analyze the paradigmatic question of connecting two Gaussian states; it will be shown that the fast-forward optimum and the full one do coincide.

## IV. ANALYTICALLY SOLVABLE SHORTCUTS: GAUSSIAN DISTRIBUTIONS

We put forward here two analytically solvable reference processes in infinite systems, $-\infty < x < \infty$. Both of them share the property of having a Gaussian distribution for all times, i.e.

$$\rho_{\rm r}(x,t) = \sqrt{\frac{\alpha(t)}{\pi}} e^{-\alpha(t)x^2}. \tag{S35}$$

A state can then be characterized by the evolving parameter $\alpha(t)$, which is proportional to the inverse of the variance of the distribution.

We introduce two different reference processes that keep the distribution Gaussian along the evolution: a free dynamics and a harmonic confinement. In these situations, the generic route via Eq. (2) is practical, i.e., it can be directly applied. For illustrative purposes though, we work out the time-mapping method via Eq. (5), which leads to the same results. Furthermore, since the dynamics in Eq. (S35) preserves the shape of the distribution, it would be possible here to use Eq. (S20) with $\mu(t) = 0$ and $\sigma(t) = \sqrt{\alpha(0)/\alpha(\Lambda(t))}$ as an alternative equivalent approach.

### A. Free diffusion

We consider the free diffusion of a Gaussian distribution as the reference process. Here, $U_{\rm r}(x) = 0$ and, given an initial $\alpha(0) = \alpha_0$, we find

$$\alpha(t) = \frac{\alpha_0}{1 + 4\alpha_0\gamma^{-1}\beta^{-1}t} \tag{S36}$$

by solving the diffusion equation. Having the reference process fully solved, the potential needed to make a time transformation $\Lambda(t)$ directly stems from Eq. (5),

$$\partial_x U(x,t) = -2\beta^{-1}\alpha_0 \frac{\dot{\Lambda}(t) - 1}{1 + 4\alpha_0\gamma^{-1}\beta^{-1}\Lambda(t)} x. \tag{S37}$$

The above expression for $\partial_x U(x,t)$ has a neat physical meaning. For $\dot{\Lambda}(t) > 1$, i.e., for an acceleration of the dynamics, this extra harmonic potential repels the particle and thus speeds up the diffusion process.

We focus on the case of an infinite acceleration, meaning $\Lambda(t_{\rm f}) \to \infty$ with finite $t_{\rm f}$. The final potential is

$$\lim_{t\to t_{\rm f}^-} \partial_x U(x,t) = -\frac{\gamma}{2} x \lim_{t\to t_{\rm f}^-} \frac{d\ln\Lambda(t)}{dt}. \tag{S38}$$

Contrarily to the situation analyzed in Sec. II, there is no critical case here. Due to the divergence of $\Lambda(t_{\rm f})$, the final potential is always singular, for arbitrary $\Lambda(t)$, since the rhs of Eq. (S38) diverges. This result is somehow intuitive: in the process defined above, our goal is to fully flatten the distribution in a finite time. This task turns to have an infinite price in terms of forcing. Note that the proof described in the main text concerning the existence of regular protocols, and detailed in Sec. II, does not conflict with the present result. The argument there is based on the existence of a normalizable stationary solution, which is not the case with the free particle over the whole real line.

### B. Harmonic potential

We next consider a time-dependent harmonic potential, $U_{\rm r}(x,t) = \beta^{-1}x^2/[2\sigma_x^2(t)]$. Note that the variance $\sigma_x^2(t)$ of the equilibrium distribution associated to the potential at time $t$ generally differs from the instantaneous variance of the evolving distribution, which is given by $[2\alpha(t)]^{-1}$. When considering the Gaussian evolution of the distribution, Eq. (S35), and the aforementioned harmonic potential, the Fokker-Planck equation for the reference process reduces to a differential equation for $\alpha(t)$,

$$\beta\gamma\frac{\dot{\alpha}(t)}{\alpha(t)} = 2\sigma_x^{-2}(t) - 4\alpha(t). \tag{S39}$$

Particularization of (5) of the main text to the harmonic case yields

$$\partial_x \Delta U(x,t) = \beta^{-1}\left(\dot{\Lambda}(t) - 1\right)\left[\sigma_x^{-2}(\Lambda(t)) - 2\alpha(\Lambda(t))\right]x. \tag{S40}$$

Interestingly, the extra potential required to manipulate the reference process is also harmonic. It is worth noting that the curvature of the potential can become negative in the time interval of interest, which may turn out to be an experimental challenge for the implementation of our time-engineered method. In particular, in order to guarantee that the harmonic potential has positive curvature, i.e., that it is confining, we need to enforce

$$\left(\dot{\Lambda}(t)-1\right)\left[\sigma_x^{-2}(\Lambda(t))-2\beta^{-1}\alpha(\Lambda(t))\right]+\sigma_x^{-2}(\Lambda(t))>0. \tag{S41}$$

This condition may limit the feasible accelerations, making a minimum—non-vanishing—connection time $t_{\mathrm{f}}$ emerge. Equation (S40) can be rewritten in an equivalent way: by comparing the rhs of Eqs. (S39) and (S40), we can write

$$\partial_x \Delta U(x,t)=\left(\dot{\Lambda}(t)-1\right)\frac{\gamma}{2}\frac{d\ln\alpha(\Lambda(t))}{d\Lambda(t)}\,x. \tag{S42}$$

To be more concrete, we look into the "static" case $\sigma_x^2(t)=\sigma_x^2$, specifically into the relaxation from one equilibrium state, with variance $\sigma_{x,0}^2=[2\alpha(0)]^{-1}\neq\sigma_x^2$, to the equilibrium state in the reference potential with variance $\sigma_x^2$. Therein, Eq. (S39) can be integrated for $\alpha^{-1}$, with the result

$$[2\alpha(t)]^{-1}=\sigma_x^2+\left(\sigma_{x,0}^2-\sigma_x^2\right)\exp\left(-\frac{2}{\gamma\beta\sigma_x^2}t\right). \tag{S43}$$

Inserting (S43) into Eq. (S42), we get

$$\partial_x \Delta U(x,t)=\left(\dot{\Lambda}(t)-1\right)\frac{1-\frac{\sigma_{x,0}^2}{\sigma_x^2}}{\beta\sigma_x^2\left[1-\frac{\sigma_{x,0}^2}{\sigma_x^2}-\exp\left(\frac{2}{\gamma\beta\sigma_x^2}\Lambda(t)\right)\right]}\,x. \tag{S44}$$

In the limit $t\to t_{\mathrm{f}}^-$, $\Lambda$ diverges and thus

$$\partial_x \Delta U(x,t_{\mathrm{f}}^-)\sim\frac{\gamma}{2}\left(1-\frac{\sigma_{x,0}^2}{\sigma_x^2}\right)\frac{d\exp\left(-\frac{2}{\gamma\beta\sigma_x^2}\Lambda(t)\right)}{dt}\,x. \tag{S45}$$

The behavior of the potential when taking the limit is governed by $\frac{d\exp\left(-\frac{2}{\gamma\beta\sigma_x^2}\Lambda(t)\right)}{dt}$, where we can identify the relaxation rate $\lambda=\frac{2}{\gamma\beta\sigma_x^2}$. This behavior is identical to that obtained when expanding in eigenfunctions, see Sec. II. Therefore, we reach here the same conclusion on the (dis)continuity at $t_{\mathrm{f}}$: the critical function $\Lambda_c(t)$ in Eq. (S25) does discriminate the "continuous" from the "discontinuous" regime.

### C. Optimal harmonic connection

Let us use the the optimal formulation developed in subsection III B to look for the optimal $\Lambda(t)\equiv g(t/t_{\mathrm{f}})$, that allows minimizing the work dissipated during the fast-forward of a reference harmonic relaxation. Our reference process evolves following Eq. (S35) and Eq. (S43). In this reference process the rate (power) of excess work can be analytically computed

$$\mathcal{P}_{\mathrm{r}}^{(\mathrm{irr})}(t)=\frac{\left[2\alpha(t)-\sigma_x^{-2}\right]^2}{2\gamma\beta^2\alpha(t)}. \tag{S46}$$

When introducing Eq. (S46) and Eq. (S43) into Eq. (S32), the differential equation for the optimal time manipulation $g$ is obtained

$$\gamma\beta\sigma_x^2\left[\sigma_x^{-2}-\left(1-e^{\frac{2}{\gamma\beta\sigma_x^2}g(s)}\right)\sigma_{x,0}^{-2}\right]g''(s)=\left[\sigma_x^{-2}-\left(1-2e^{\frac{2}{\gamma\beta\sigma_x^2}g(s)}\right)\sigma_{x,0}^{-2}\right]g'(s)^2. \tag{S47}$$

It has a unique real solution when submitted to the boundary conditions, $g(0)=0$ and $\lim_{s\to1}g(s)=\infty$, which is

$$g(s)=\frac{\gamma\beta\sigma_x^2}{2}\ln\left[\frac{\sigma_x^{-2}-\sigma_{x,0}^{-2}}{(1-s)\left\{\sigma_x^{-2}-\sigma_{x,0}^{-2}+\left[2\sqrt{\sigma_{x,0}^{-2}\sigma_x^{-2}}-\left(\sigma_{x,0}^{-2}+\sigma_x^{-2}\right)\right]s\right\}}\right]. \tag{S48}$$

Remarkably, the evolution for the variance of the optimal evolution, which is obtained when introducing Eq. (S48) into Eq. (S43), yields

$$[2\alpha(\Lambda(t))]^{-1} = \left[\sigma_{x,0} + \left(\sigma_x - \sigma_{x,0}\right)\frac{t}{t_\mathrm{f}}\right]^2, \tag{S49}$$

which is the full optimal protocol found in the literature [1] resulting in an optimal irreversible work

$$\beta W_\mathrm{opt}^{(\mathrm{irr})} = \frac{\gamma\beta\sigma_x^2}{t_\mathrm{f}}\left(1 - \frac{\sigma_{x,0}}{\sigma_x}\right)^2. \tag{S50}$$

Thus, the optimization of our fast-forward protocol recovers the full optimal protocol for the paradigmatic case of harmonic connections. The reason is that full optimization yields a sequence of intermediate states that are all Gaussian, a common feature with the fast-forward evolution in a harmonic potential $U_\mathrm{r}$.

### D. Comparing the costs of the FF and the full optimal processes

It is important to underscore here that one of our main concerns when introducing our fast-forward procedure was the regularity of the driving protocol. The optimal protocol reobtained above develops finite jumps in the potential at initial and final times. The prize of the regularization of such jumps involves an unavoidable increase of the irreversible work. Such an extra cost can be minimized by optimizing the fast-forward procedure within the family of functions given by Eq. (6) in the main text. Once that the characteristic time $\tau$ and the final time $t_\mathrm{f}$ are fixed, the optimization problem is just over the parameter $\zeta$. Taking the function $\Lambda(t)$ proposed in the main text with $\tau = \lambda_1^{-1} = \gamma\beta\sigma_x^2$, and using Eq. (S43), Eq. (S46) and (S31), we obtain

$$\beta W^{(\mathrm{irr})} = \frac{\gamma\beta\sigma_x^2}{t_\mathrm{f}}\int_0^1 ds\, \frac{\left(1 - \frac{\sigma_{x,0}^2}{\sigma_x^2}\right)^2 \exp\left[-2s^2(1-s)^{-\zeta}\right] s^2(1-s)^{-2\zeta-2}[2+s(\zeta-2)]^2}{\frac{\sigma_{x,0}^2}{\sigma_x^2} - 1 + \exp\left[2s^2(1-s)^{-\zeta}\right]}. \tag{S51}$$

The fraction $W^{(\mathrm{irr})}/W_\mathrm{opt}^{(\mathrm{irr})}$ only depends on the contraction rate $\sigma_{x,0}/\sigma_x$ and the parameter $\zeta$, since the excess works in both protocols have the same scaling properties. This fraction is displayed, for $\sigma_{x,0}/\sigma_x = 0.1$ and $\sigma_{x,0}/\sigma_x = 10$, in Fig. S2. It follows that optimal values of the parameter $\zeta$ appear, $\zeta \simeq 0.15$ and $\zeta \simeq 0.28$, for which $W^{(\mathrm{irr})}/W_\mathrm{opt}^{(\mathrm{irr})} \simeq 1.12$ and $W^{(\mathrm{irr})}/W_\mathrm{opt}^{(\mathrm{irr})} \simeq 1.26$, for the two compression rates considered respectively. Besides, optimizing simultaneously on $\tau$ and $\zeta$ brings down these values to 1.04 and 1.13, respectively. Therefore, our regular FF protocols come at a cost that only slightly exceed the absolute minimal one.

## V. EXPANSIONS IN THE EIGENFUNCTIONS OF THE REFERENCE RELAXATION PROCESS

In the following, we explicitly provide the eigenvalues and eigenfunctions for the Hamiltonian operator defined in the main text in the cases of either free, $U_\mathrm{r}(x) = 0$, or harmonic, $U_\mathrm{r}(x) = \frac{x^2}{2\beta\sigma_x^2}$, reference potentials. The corresponding relaxations are the reference processes that we have considered to illustrate our time-engineered procedure (fast- or slow-forward, fast- or slow-backward, welding method of Fig. 1). The mathematical problem amounts to looking for the possible eigenvalues, $\lambda_n$, and eigenfunctions, $\varphi_n(x)$, of Schrödinger's equation

$$\left\{-\frac{1}{\gamma\beta}\partial_x^2 + \frac{1}{2\gamma}\left[\frac{\beta U_\mathrm{r}'(x)^2}{2} - U_\mathrm{r}''(x)\right]\right\}\varphi_n(x) = \lambda_n\varphi_n(x). \tag{S52}$$

The boundary conditions

$$\left[\frac{1}{2}\varphi(x)\partial_x U_\mathrm{r}(x) + \beta^{-1}\partial_x\varphi_n(x)\right]_{x=x_b} = 0 \tag{S53}$$

come from the cancellation of the probability current at the boundary $x_b$ of the system. This condition further simplifies in the cases analyzed below.

The stationary solution $\varphi_0 \propto \exp^{-\beta U_\mathrm{r}(x)}$ is associated to the vanishing eigenvalue. In the following, we focus on the rest of the spectrum.

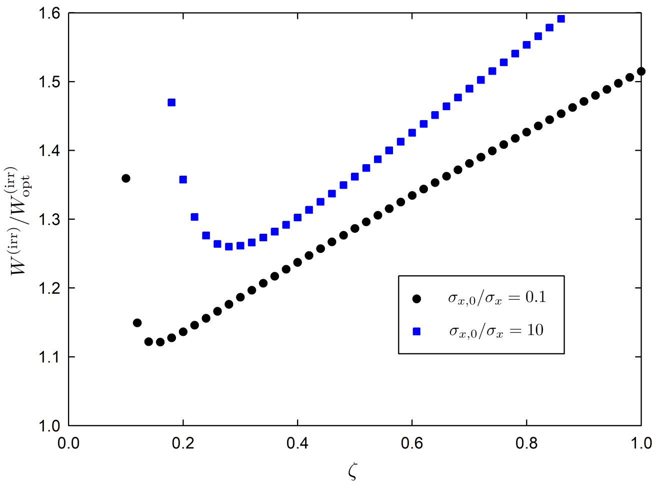


FIG. S2. Energetic cost of fast-forward protocols (in terms of the irreversible work) for a 10-fold expansion and a 10-fold compression ($\sigma_{x,0}/\sigma_x = 0.1$ and $\sigma_{x,0}/\sigma_x = 10$). The cost is normalized by the full optimal value. The ratio is plotted as a function of the parameter $\zeta$, with $\Lambda(t)$ given by Eq. (6) of the main text. The optimal value of the irreversible work (within the FF family chosen) is quite close to the full minimum—around 12 % larger in the expansion considered, and 26% for the compression.

### A. Free dynamics

Let us start with the simple case of a free particle, $U_{\mathrm{r}}(x) = 0$, in a finite box $x \in [0, L]$. We have to solve

$$-\frac{1}{\gamma\beta}\partial_x^2\varphi_n(x) = \lambda_n\varphi_n(x) \qquad \text{with the Neumann boundary condition} \qquad \partial_x\varphi_n(x) = 0. \tag{S54}$$

The spectrum of this standard problem is given by the trigonometric family

$$\varphi_n(x) = \sqrt{\frac{2}{L}}\cos\left(\frac{n\pi}{L}x\right), \quad \text{with } \lambda_n = \frac{n^2\pi^2}{\gamma\beta L^2}, \quad \text{for } n = 1, 2, \ldots. \tag{S55}$$

The relaxation reference process considered in the main text starts from an exponential distribution $\rho_{\mathrm{r}}(x, 0) \propto \exp(\beta F x)$. Defining the dimensionless variables

$$\tilde{x} = \frac{x}{L}, \quad \tilde{t} = \lambda_1 t, \tag{S56}$$

and expanding the reference process in its eigenfunctions, we end up with

$$\tilde{\rho}_{\mathrm{r}}(\tilde{x}, \tilde{t}) = 1 + \frac{2\beta F L}{e^{\beta F L} - 1}\sum_{n=1}^{\infty}\cos(n\pi\tilde{x})e^{-n^2\tilde{t}}\int_0^1 d\tilde{x}'\cos(n\pi\tilde{x}')e^{\beta F L\tilde{x}'} \tag{S57}$$

where we have taken into account that, after the change of variables, the corresponding distributions are related by $\tilde{\rho}_{\mathrm{r}}(\tilde{x}, \tilde{t}) = L\rho_{\mathrm{r}}(x, t)$.

### B. Harmonic potential

What is required here is the spectrum of the harmonic potential, corresponding to

$$\left\{-\frac{1}{\gamma\beta}\partial_x^2 + \frac{1}{2\gamma\beta\sigma_x^2}\left[\frac{x^2}{2\sigma_x^2} - 1\right]\right\}\varphi_n(x) = \lambda_n\varphi_n(x). \tag{S58}$$

With the correspondence $\frac{1}{\gamma\beta} \to \frac{\hbar^2}{2m}$ and $(2\gamma\beta\sigma_x^4)^{-1} \to m\omega^2$, we get the equation of the traditional quantum harmonic oscillator with the energy spectrum shifted by $-\hbar\omega/2$. Using the solution of the quantum harmonic oscillator, we get

$$\varphi_n(x) = \sqrt{\frac{1}{2^n n! \sqrt{2\pi\sigma_x^2}}} H_n\left(\frac{x}{\sqrt{2\sigma_x^2}}\right) e^{-\frac{x^2}{4\sigma_x^2}}, \quad \text{with } \lambda_n = \frac{n}{\gamma\beta\sigma_x^2}, \quad \text{for } n = 0, 1, 2, \ldots. \tag{S59}$$

For studying the relaxation reference process, we start from an arbitrary initial distribution $\rho_{\mathrm{r}}(x) = Z_{\mathrm{i}}^{-1} e^{-\beta U_{\mathrm{i}}(x)}$. Introducing the dimensionless variables,

$$\tilde{x} = \frac{x}{\sqrt{2\sigma_x^2}}, \quad \tilde{t} = \lambda_1 t, \tag{S60}$$

we can carry out the expansion of the reference distribution. This results in

$$\tilde{\rho}_{\mathrm{r}}(\tilde{x}, \tilde{t}) = \frac{e^{-\tilde{x}^2}}{\sqrt{\pi}} \left[1 + \sum_{n=1}^{\infty} \frac{I_n}{2^n n!} H_n(\tilde{x}) e^{-n\tilde{t}}\right] \tag{S61}$$

with

$$I_n = \frac{\sqrt{2\sigma_x^2}}{Z_{\mathrm{i}}} \int_{-\infty}^{\infty} dx H_n(x) e^{-\beta U_{\mathrm{i}}\left(\sqrt{2\sigma_x^2}x\right)}, \tag{S62}$$

and $\tilde{\rho}_{\mathrm{r}}(\tilde{x}, \tilde{t}) = \sqrt{2\sigma_x^2}\rho_{\mathrm{r}}(x, t)$. Note that in the cases illustrated in the main text, where the initial state can be parametrized solely by its variance, $I_n$ becomes a function of the ratio between the variance of such a state and $\sigma_x^2$.

For the sake of completeness, we accompany this SM with a Mathematica notebook where the welding driving leading to Fig. 3 is computed.

## VI. CONVERGENCE OF THE EXPANSION IN EIGENFUNCTIONS OF THE REFERENCE POTENTIAL

In this section, we discuss the reduction of the error made in the fast-forward protocol when increasing the cutoff used in the expansion in the basis of eigenfunctions. To do so, we have computed the distance between the target final state $\rho_{\mathrm{f}}(x) = 1$ and the state reached at the final time in the truncated fast-forward protocol $\rho_{\mathrm{FF}}(x, t_{\mathrm{f}})$, for the process illustrated in Fig. 2 of the main text. The state reached in the truncated fast-forward protocol can be computed numerically solving the Fokker-Planck equation, submitted to the initial condition, with the potential $U(x, t)$ obtained from Eq. (5) after introducing the truncation of $\rho_{\mathrm{r}}(x, t)$ in Eq. (8). For measuring the distance, we use the norm

$$\left\|\rho_{\mathrm{f}}(x) - \rho_{\mathrm{FF}}(x, t_{\mathrm{f}})\right\| = \sqrt{\int_{\mathcal{D}} dx \left[\rho_{\mathrm{f}}(x) - \rho_{\mathrm{FF}}(x, t_{\mathrm{f}})\right]^2}. \tag{S63}$$

This distance depends on the cutoff $n_{cut}$, since the truncation affects $\rho_{\mathrm{FF}}(x, t_{\mathrm{f}})$.

We show the results regarding the improvement of the convergence with the cutoff in Fig. S3: an exponential improvement is observed. The error made due to the truncation is small, already for moderate values for the cutoff. Yet, in the main text, we used a somewhat larger value $n_{cut} = 70$, to avoid spurious oscillations affecting the force field at very short times. These oscillations, which do not affect the quality of the final state reached, are present at early times only and are akin to the so-called Gibbs phenomenon [11].

## VII. FAST-FORWARD PROTOCOLS IN DIMENSION $d$

For simplicity, we have presented our results in one spatial dimension. Generalization to higher dimensions is not straightforward, although an operational formalism has been recently proposed [12], and could be put to work. For a radially symmetric situation, the problem simplifies: the Fokker-Planck equation reads

$$\gamma\partial_t \rho(r, t) = r^{1-d}\partial_r \left\{r^{d-1}\left[\rho(r, t)\partial_r U(r, t) + \beta^{-1}\partial_r \rho(r, t)\right]\right\}, \tag{S64}$$

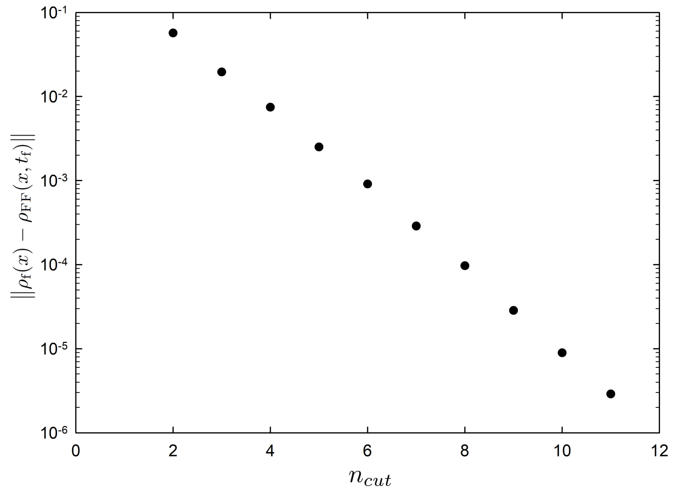


FIG. S3. Convergence of the truncated fast-forward protocol for the situation displayed in Fig. 2. The distance between the target state and the output of the algorithm, using the norm in Eq.(S63), is displayed as a function of the number of terms used in the expansion, $n_{cut}$. The error is approximately reduced ten-fold for each two extra terms that are added in the expansion.

which can be recast, using the velocity field $v(r,t) = -\gamma^{-1}\left[\partial_r U(r,t) + \beta^{-1}\partial_r \ln\rho(r,t)\right]$, as

$$\partial_t \rho(r,t) = -r^{1-d}\partial_r \left[r^{d-1} v(r,t)\rho(r,t)\right]. \tag{S65}$$

If the problem is defined within a sphere of radius $R$, we can write

$$v(r,t) = -\frac{r^{1-d}}{\rho(r,t)}\partial_t \int_R^r dr' r'^{d-1}\rho(r',t), \tag{S66}$$

where we have integrated from $R$ to $r < R$ using natural boundary conditions, i.e., vanishing current, at the shell of radius $R$. If $\rho(r,t) = \rho_{\mathrm{r}}(r,\Lambda(t))$ is given by a time manipulation of a reference solution for a certain $v_r(r,t)$, we reach the same relation than in the one-dimensional case,

$$v(r,t) = \dot{\Lambda}(t) v_{\mathrm{r}}(t,\Lambda(t)). \tag{S67}$$

Hence, the potential for performing the time manipulation is given by

$$\Delta U(r,t) \equiv \partial_r\left[U(r,t) - U_{\mathrm{r}}(r,\Lambda(t))\right] = \left(1 - \dot{\Lambda}(t)\right)\gamma v_{\mathrm{r}}(r,\Lambda(t)), \tag{S68}$$

also in complete analogy with the 1-dimensional expression derived in the main text.

In the spherically symmetric case, an alternative way of relating the solution to the one-dimensional case stems from considering the radial probability (proportional to) $r^{d-1}\rho(r,t)$, instead of the "volumetric" probability density function $\rho(r,t)$. The former obeys a one-dimensional Fokker-Planck equation with an effective potential $U_{\mathrm{eff}}(r,t) = U(r,t) + \beta^{-1}(1-d)\ln r$.


[1] T. Schmiedl and U. Seifert, Phys. Rev. Lett. **98**, 108301 (2007).
[2] I. A. Martínez, A. Petrosyan, D. Guéry-Odelin, E. Trizac, and S. Ciliberto, Nature Physics **12**, 843 (2016).
[3] Y. Zhang, EPL (Europhysics Letters) **128**, 30002 (2019).
[4] Y. Zhang, Journal of Statistical Physics **178**, 1336 (2020).
[5] S. Martínez-Garaot, M. Palmero, J. G. Muga, and D. Guéry-Odelin, Phys. Rev. A **94**, 063418 (2016).
[6] S. Ciliberto, Phys. Rev. X **7**, 021051 (2017).
[7] In other words, the time integral of $\mathcal{P}_{\mathrm{r}}^{(\mathrm{irr})}(t)$ gives the average irreversible work for the reference process.
[8] E. Aurell, C. Mejía-Monasterio, and P. Muratore-Ginanneschi, Phys. Rev. Lett. **106**, 250601 (2011).

[9] E. Aurell, C. Mejía-Monasterio, and P. Muratore-Ginanneschi, Phys. Rev. E **85**, 020103 (2012).
[10] E. Aurell, K. Gawędzki, C. Mejía-Monasterio, R. Mohayaee, and P. Muratore-Ginanneschi, Journal of Statistical Physics **147**, 487 (2012).
[11] See chapter IX of Ref. [13] for a detailed account of the Gibbs phenomenon in Fourier series.
[12] A. G. Frim, A. Zhong, S.-F. Chen, D. Mandal, and M. R. DeWeese, Phys. Rev. E **103**, L030102 (2021).
[13] H. S. Carslaw, *Introduction to the theory of Fourier's series and integrals* (Dover Publications, New York, 1950).
